# Supplementary material for: Reconstructing Training Data from Model Gradient, Provably
Source: arXiv:2212.03714 source file (2023-06-10)
Supplement: Supplementary file 1 [file non_uniform.tex]

\section{Non Uniform Samples}
\label{sec:nonuni}
In Theorem \ref{thm:npm}, we have assumed that the training samples $\{\bx_i\}$ should be drawn uniformly from the unit ball $\mathcal{S}^{d-1}$. In this section, we relax the restriction and prove that a similar error bound is true with non uniform i.i.d. samples. To achieve this goal, we will use a different technique of tensor decomposition introduced by Algorithm 1 from \citep{recovery}. 

First we estimated the orthogonal span $U$ of training samples $\{\bx_i|i\in B\}$ with power method and denoted by $V$. Then we can conduct noisy tensor decomposition to $T(V,V,V)$ with Algorithm 1 in \citep{kuleshov2015tensor} and have $\{s_i\bu_i\}_{i=1}^B$ as an estimation of $\{V^\top \bx_i\}_{i=1}^B$, where $s_i$ are unknown signs. Finally, we can use Algorithm 4 in \citep{recovery} to recover $s_i$ and $r_i^*$ and eventually recover $\bx_i$ and $y_i$.

Formally, following the proof of Theorem 5.6 in \citep{recovery}, we have
\begin{equation}
\begin{aligned}
\left\|\bx_i-s_i V \bu_i\right\| & \leq\left\| V V^{\top}\bx_i-\bw_i\right\|+\left\|V V^{\top} \bw_i-V s_i \bu_i\right\| \\
&=\left\|V V^{\top} \bw_i-\bw_i\right\|+\left\|V^{\top} \bw_i-s_i \bu_i\right\|.
\end{aligned}
\end{equation}

For the first term, we have
\begin{equation}
    \|VV^\top\bx_i-\bx_i\|\le \Tilde{O}(\frac{B\sqrt{d}}{|\nu|\sqrt{m}})
\end{equation}
by Lemma E.6 in \citep{recovery}, Proposition \ref{matrix} and Remark \ref{rmk:2bound}, where $\nu=\mathbb{E}_{z\in\mathcal{N}(0,1)}\sigma''(z)$ if it is not 0 and $\nu=\lambda$ otherwise.
For the second term, we have
\begin{equation}
    \|V^\top\bx_i-s_i\bu_i\|\le\Tilde{O}(\frac{B^3}{|\lambda|\sqrt{m}})
\end{equation}
by Theorem 3 in \citep{kuleshov2015tensor} and Proposition \ref{prop:V}. Thus, if $d\gg B$, we have $\sqrt{\frac{1}{B}\sum_{i=1}^B\|\bx_i-\hat{\bx_i}\|^2}\le\Tilde{O}(\frac{\sqrt{d}}{\sqrt{m}})$.
